# Supplementary material for: OmniPhys: Knowledge-Graph-Driven Benchmarking and Collective Optimization for Physical Commonsense in Text-to-Image Generation
Source: arXiv:2607.25641 source file (2026-07-28)
Supplement: Supplementary file 1 [file appendix_1.tex]

\section{End-to-End Illustration of OmniPrompt}
\label{app:running-example}

This appendix complements Section~\ref{sec:omniprompt}.
We instantiate \textbf{one optimization step} with batch size $B=2$ and ensemble size $N=4$, using the notation of the main text:
query index $i$, image index $j$, enhanced prompt $\tilde{x}_i=\mathcal{L}(x_i;P^{(t)})$, collective buffer $e_i=\langle \bar{S}_i, \mathcal{R}_i \rangle$ (Eq.~\ref{eq:collective-feedback}), unified gradient $g_{\tilde{x}}$ (Eq.~\ref{eq:unified-gradient}), meta-gradients $\{g_{P}^{(i)}\}_{i=1}^{B}$ (Eq.~\ref{eq:meta-gradient}), and update $P^{(t+1)}=\Phi(P^{(t)};\{g_{P}^{(i)}\}_{i=1}^{B})$ (Eq.~\ref{eq:policy-update}).
Modules $\mathcal{G}$ and $\mathcal{E}$ are external to the TextGrad graph; only $\mathcal{L}$ and $P$ participate in $\Gamma$.
Fixed templates are quoted verbatim from our implementation; instantiated values are taken from a real training log.

\paragraph{Component map.}
\begin{center}
\small
\begin{tabular}{lll}
\toprule
\textbf{Symbol} & \textbf{Role} & \textbf{Implementation} \\
\midrule
$P$ & Meta-Policy & \texttt{system\_prompt\_var} \\
$\mathcal{L}$ & Prompt Enhancer & GPT-4o (\texttt{BlackboxLLM}) \\
$\mathcal{G}$ & Stochastic T2I Manifold & Janus-Pro-7B \\
$\mathcal{E}$ & Multimodal Evaluator & Gemini-2.5-Pro \\
$\Gamma$ & Feedback Calculator & TextGrad backward engine (GPT-4o) \\
$\Phi$ & Meta-Policy Optimizer & Textual Gradient Descent (GPT-4o) \\
\bottomrule
\end{tabular}
\end{center}

\subsection{Fixed Instruction Templates}
\label{app:fixed-prompts}

\subsubsection{Initial Meta-Policy $P^{(0)}$ (Reasoning-before-Synthesis)}
\label{app:meta-policy-init}
System message for $\mathcal{L}$ in the forward pass (Section~\ref{sec:reasoning-before-synthesis}).

\begin{lstlisting}[caption={Initial meta-policy $P^{(0)}$.},label={lst:meta-policy-init}]
You are a prompt expander for image generation. Given a simple input prompt, your job is to expand it into a rich, physically plausible, visually descriptive sentence that guides image models to generate accurate and realistic scenes. Step 1: Reason about the implicit physical states of objects in the prompt. Think through what physical principles are involved and how they influence the object's behavior. Step 2: Generate the expanded descriptive text. Combine the original prompt with the physical insights from Step 1 to produce a rich, coherent, and visually specific description -- optimized for image generation. Finally, output your expanded text in JSON format {"expanded_text": "The final expanded text for image generation -- descriptive, concrete, and physics-aware."}
\end{lstlisting}

\subsubsection{Multimodal Evaluator $\mathcal{E}$}
\label{app:evaluator-instruction}
(Section~\ref{sec:diagnostic-eval}).
For each image $I_{i,j}$, the system appends PKG-annotated physical state descriptions and parses \texttt{Score: [0|1]. Reason: [...]}.

\begin{lstlisting}[caption={Fixed instruction for $\mathcal{E}$.},label={lst:evaluator}]
You are an expert multi-modal AI specializing in physics-based image analysis. Your task is to act as a strict referee for image plausibility.

You will be provided with:
1. A generated image.
2. A set of text descriptions detailing the expected physical states and behaviors of objects in the image.

Your evaluation process must be as follows:
1. **Analyze the Image vs. Descriptions**: Carefully compare the visual content of the image against EACH of the provided physical state descriptions.
2. **Make a Final Judgment**: Based on your analysis, determine if the image, as a whole, is physically plausible and correctly represents the described states.
3. **Provide a Structured Output**: You MUST format your response STRICTLY as follows:

Score: [SCORE]. Reason: [REASON]

**Formatting Rules**:
- **[SCORE]**: This must be either `1` or `0`.
  - Use `1` if the image is physically plausible and fully consistent with ALL descriptions.
  - Use `0` if the image violates ANY of the physical descriptions or exhibits any other obvious commonsense errors.
- **[REASON]**: This is a concise, one-sentence explanation for your score.
  - If the score is 1, the reason should be a positive confirmation.
  - If the score is 0, the reason must clearly and specifically state the most significant violation.
\end{lstlisting}

After per-image audits, the trainer aggregates $\{s_{i,j}, r_{i,j}\}_{j=1}^{N}$ into $e_i$ (Eq.~\ref{eq:collective-feedback}).

\subsubsection{Feedback Calculator $\Gamma$}
\label{app:gamma-templates}

\paragraph{String-function purpose (Stage 1 of $\Gamma$).}
\begin{lstlisting}[caption={Function purpose for computing $g_{\tilde{x}}$.},label={lst:gamma-purpose}]
This function processes a batch of text predictions. The function's output (the 'value') is a concatenated string of comprehensive feedback summaries, separated by '---'.

Each summary has the format: 'Score: [SCORE]. Reason: [REASON]'.

**Interpreting the [SCORE]**:
- The [SCORE] is a float number between 0.0 and 1.0, representing the success rate (physical plausibility) of images generated from a single prediction.
- A score of **1.0** is perfect. The gradient should be minimal, suggesting no change or only minor reinforcement.
- A score of **0.0** is a complete failure. The gradient should be strongly corrective, focusing on the provided failure reasons.
- A score **between 0.0 and 1.0** indicates partial success. The gradient should be moderately corrective, with its strength proportional to how far the score is from 1.0.
\end{lstlisting}

\paragraph{Backward engine system prompt.}
\begin{lstlisting}[caption={System prompt for all $\Gamma$ backward calls.},label={lst:backward-system}]
You are part of an optimization system that improves a given text (i.e. the variable). You are the gradient (feedback) engine. Your only responsibility is to give intelligent and creative feedback and constructive criticism to variables, given an objective specified in <OBJECTIVE_FUNCTION> </OBJECTIVE_FUNCTION> tags. The variables may be solutions to problems, prompts to language models, code, or any other text-based variable. Pay attention to the role description of the variable, and the context in which it is used. You should assume that the variable will be used in a similar context in the future. Only provide strategies, explanations, and methods to change in the variable. DO NOT propose a new version of the variable, that will be the job of the optimizer. Your only job is to send feedback and criticism (compute 'gradients'). For instance, feedback can be in the form of 'Since language models have the X failure mode...', 'Adding X can fix this error because...', 'Removing X can improve the objective function because...', 'Changing X to Y would fix the mistake ...', that gets at the downstream objective.
If a variable is already working well (e.g. the objective function is perfect, an evaluation shows the response is accurate), you should not give feedback.
\end{lstlisting}

\paragraph{User template: $e \rightarrow g_{\tilde{x}}$.}
\begin{lstlisting}[caption={String-function backward template.},label={lst:gamma-stage1}]
You will give feedback to a variable with the following role: <ROLE> {variable_desc} </ROLE>. Here is an evaluation of the variable using a string-based function:

Function purpose: {function_purpose}

<INPUTS_TO_FUNCTION> {inputs_string} </INPUTS_TO_FUNCTION>

<OUTPUT_OF_FUNCTION> {response_value} </OUTPUT_OF_FUNCTION>

<OBJECTIVE_FUNCTION>Your goal is to give feedback and criticism to the variable given the above evaluation output. Our only goal is to improve the above metric, and nothing else. </OBJECTIVE_FUNCTION>

We are interested in giving feedback to the {variable_desc} for this conversation. Specifically, give feedback to the following span of text:

<VARIABLE> {variable_short} </VARIABLE>

Given the above history, describe how the {variable_desc} could be improved to improve the <OBJECTIVE_FUNCTION>. Be very creative, critical, and intelligent.
\end{lstlisting}

\paragraph{User template: $g_{\tilde{x}} \rightarrow g_{P}^{(i)}$.}
\begin{lstlisting}[caption={LLM-chain backward template.},label={lst:gamma-stage2}]
You will give feedback to a variable with the following role: <ROLE> {variable_desc} </ROLE>. Here is a conversation with a language model (LM):

<LM_SYSTEM_PROMPT> {system_prompt} </LM_SYSTEM_PROMPT>

<LM_INPUT> {prompt} </LM_INPUT>

<LM_OUTPUT> {response_value} </LM_OUTPUT>

This conversation is part of a larger system. The <LM_OUTPUT> was later used as {response_desc}.

<OBJECTIVE_FUNCTION>Your goal is to give feedback to the variable to address the following feedback on the LM_OUTPUT: {response_gradient} </OBJECTIVE_FUNCTION>

We are interested in giving feedback to the {variable_desc} for this conversation. Specifically, give feedback to the following span of text:

<VARIABLE> {variable_short} </VARIABLE>

Given the above history, describe how the {variable_desc} could be improved to improve the <OBJECTIVE_FUNCTION>. Be very creative, critical, and intelligent.
\end{lstlisting}

\subsubsection{Meta-Policy Optimizer $\Phi$}
\label{app:phi-templates}

\begin{lstlisting}[caption={Optimizer system prompt ($\Phi$).},label={lst:phi-system}]
You are part of an optimization system that improves text (i.e., variable). You will be asked to creatively and critically improve prompts, solutions to problems, code, or any other text-based variable. You will receive some feedback, and use the feedback to improve the variable. The feedback may be noisy, identify what is important and what is correct. Pay attention to the role description of the variable, and the context in which it is used. This is very important: You MUST give your response by sending the improved variable between {new_variable_start_tag} {improved variable} {new_variable_end_tag} tags. The text you send between the tags will directly replace the variable.
\end{lstlisting}

\begin{lstlisting}[caption={Optimizer user prompt template ($\Phi$).},label={lst:phi-user}]
Here is the role of the variable you will improve: <ROLE>{variable_desc}</ROLE>.

The variable is the text within the following span: <VARIABLE> {variable_short} </VARIABLE>

Here is the context and feedback we got for the variable:

<CONTEXT>{variable_grad}</CONTEXT>

Improve the variable ({variable_desc}) using the feedback provided in <FEEDBACK> tags.

Send the improved variable in the following format:

<IMPROVED_VARIABLE>{the improved variable}</IMPROVED_VARIABLE>

Send ONLY the improved variable between the <IMPROVED_VARIABLE> tags, and nothing else.
\end{lstlisting}

\subsection{Running Example ($B=2$, $N=4$)}
\label{app:stages}

\subsubsection{Stage I: Prompt Enhancement ($\mathcal{L}$)}
\label{app:stage1}
Given $P^{(0)}$ (Listing~\ref{lst:meta-policy-init}), $\mathcal{L}$ produces:

\begin{center}
\small
\begin{tabular}{cl}
\toprule
& Query $x_i$ \\
\midrule
$x_1$ & \textit{An inflatable toy filled with helium is placed in a sealed carbon dioxide-filled room.} \\
$x_2$ & \textit{A plastic bag filled with sulfur hexafluoride is placed in a sealed hydrogen-filled room.} \\
\bottomrule
\end{tabular}
\end{center}

\begin{lstlisting}[caption={$\tilde{x}_1 = \mathcal{L}(x_1; P^{(0)})$ (abbreviated).},label={lst:x1}]
{"expanded_text": "A brightly colored inflatable toy, shaped like a balloon animal, is filled with helium and floats gently in the air. It is placed in a sealed room filled with a dense, colorless carbon dioxide gas. The toy hovers near the ceiling, buoyed by the lighter helium inside it, while the heavier carbon dioxide gas pools closer to the floor, creating a subtle gradient in the room's atmosphere. ..."}
\end{lstlisting}

$\tilde{x}_2$ analogously describes a plastic bag of SF$_6$ in a hydrogen-filled room.
The batch input to $\Gamma$ is $\bigoplus_{i=1}^{B}\tilde{x}_i$ (separator: \texttt{---}).

\subsubsection{Stage II: Visual Synthesis and Diagnostic Evaluation ($\mathcal{G}$, $\mathcal{E}$)}
\label{app:stage2}
For each $\tilde{x}_i$, $\mathcal{G}$ samples $\mathcal{I}_i=\{I_{i,1},\ldots,I_{i,N}\}$ with $N=4$.
For each $I_{i,j}$, $\mathcal{E}$ returns $(s_{i,j}, r_{i,j})$ and forms $e_i$ (Eq.~\ref{eq:collective-feedback}).
Example buffer for $x_1$:

\begin{lstlisting}[caption={Collective feedback buffer $e_1$.},label={lst:e1}]
Score: 0.50. Reason: The model's output consistency was evaluated on 4 samples, with 2 successes.
Observed physical violations include:
- The inflatable toy is visibly suspended by a string attached to the ceiling, which contradicts the description that it has no visible support or attachment.
- An inflatable toy filled with air would fall due to gravity, and one filled with a lighter-than-air gas would rise to the ceiling; it would not hover unsupported in the middle of the room.
\end{lstlisting}

Here $\bar{S}_1=\frac{1}{4}\sum_{j=1}^{4}s_{1,j}=0.50$.
An analogous buffer $e_2$ is built for $x_2$.
The batch feedback passed to $\Gamma$ is $\bigoplus_{i=1}^{B} e_i$.

\subsubsection{Stage III: TextGrad Loss Node}
\label{app:stage3}
The loss node binds $\bigoplus_{i=1}^{B}\tilde{x}_i$ to $\bigoplus_{i=1}^{B} e_i$ using the function purpose in Listing~\ref{lst:gamma-purpose}.
This node is the root of backward propagation; $\mathcal{G}$ and $\mathcal{E}$ are not part of this graph.

\subsubsection{Stage IV: Feedback Derivation ($\Gamma$)}
\label{app:stage4}

\paragraph{Step 1: Unified prompt-level gradient.}
One string-function backward yields $g_{\tilde{x}}$ (Listings~\ref{lst:backward-system} and~\ref{lst:gamma-stage1}):

\begin{lstlisting}[caption={$g_{\tilde{x}}$ (excerpt).},label={lst:gx}]
To improve the variable and achieve a higher score in the evaluation metric, the following feedback and criticism are provided:

1. **Addressing Physical Plausibility Issues**:
   - The description of the inflatable toy hovering unsupported in the middle of the room is physically implausible. To improve, the text should explicitly describe a mechanism or context that justifies this behavior. For example:
     - If the toy is described as "hovering," the text should mention magnetic levitation, fan-based suspension, or another plausible technology.
     - Alternatively, if filled with a lighter-than-air gas, the text should clarify tethering to the ceiling rather than "hovering unsupported."
   - Removing or rephrasing "no visible support or attachment" would eliminate contradictions flagged by $\mathcal{E}$.
2. **Consistency in Descriptions**: ...
\end{lstlisting}

$g_{\tilde{x}}$ is broadcast to each branch $\tilde{x}_i$ via idempotent concatenation backward.

\paragraph{Step 2: Meta-level gradients.}
For each query $i$, LLM-chain backward (Listing~\ref{lst:gamma-stage2}) yields $g_{P}^{(i)}$:

\begin{lstlisting}[caption={$g_{P}^{(1)}$ (excerpt).},label={lst:gp1}]
1. **Explicit Emphasis on Physical Plausibility**:
   - The system prompt should explicitly instruct the LLM to prioritize physical plausibility in its reasoning and output. Adding a directive like, "Ensure that all described phenomena are consistent with real-world physical laws and provide mechanisms or context to justify any unusual or unexpected behaviors," would help address implausible descriptions (e.g., unsupported hovering).

2. **Encouraging Mechanistic Explanations**:
   - After Step 1, require the LLM to reason about and describe mechanisms that justify object behavior (e.g., buoyancy, tethering, magnetic levitation).
\end{lstlisting}

A second gradient $g_{P}^{(2)}$ is derived from $x_2$ analogously.

\subsubsection{Stage V: Meta-Policy Update ($\Phi$)}
\label{app:stage5-update}
$\Phi$ aggregates $\{g_{P}^{(i)}\}_{i=1}^{B}$ into one TGD prompt (Listings~\ref{lst:phi-system}--\ref{lst:phi-user}) and produces $P^{(t+1)}$.
Key addition in Step~1 of $P^{(t+1)}$:

\begin{lstlisting}[caption={Updated Step~1 in $P^{(t+1)}$ (excerpt).},label={lst:p-update}]
Step 1: Reason about the implicit physical states of objects in the prompt. Think through what physical principles are involved and how they influence the object's behavior. Ensure that all described phenomena adhere to real-world physical laws, and provide mechanisms or context to justify any unusual or unexpected behaviors.
\end{lstlisting}

\paragraph{Summary flow.}
\begin{center}
\small
\begin{tabular}{cll}
\toprule
\textbf{Stage} & \textbf{Module} & \textbf{Output} \\
\midrule
I   & $\mathcal{L}(x_i; P^{(t)})$ & $\tilde{x}_i$ \\
II  & $\mathcal{G}(\tilde{x}_i)$, $\mathcal{E}(I_{i,j})$ & $e_i=\langle \bar{S}_i, \mathcal{R}_i \rangle$ \\
III & TextGrad loss node & backward root \\
IV  & $\Gamma$ & $g_{\tilde{x}}$, $\{g_{P}^{(i)}\}_{i=1}^{B}$ \\
V   & $\Phi$ & $P^{(t+1)}$ \\
\bottomrule
\end{tabular}
\end{center}

\endgroup % 结束 lstset 局部作用域
